# Supplementary material for: Electronic transport in double-nanowire superconducting islands with multiple terminals
Source: arXiv:2203.09213 ancillary file (2022-03-17)
Supplement: Supplementary file 1 [file DNW_SI_Supplemental_Information.pdf]

# Supplemental Material: Electronic transport in double-nanowire superconducting islands with multiple terminals

Alexandros Vekris[1,2], Juan Carlos Estrada Saldaña[1], Thomas Kanne[1], Mikelis Marnauza[1], Dags Olsteins[1], Matteo M. Wauters[1,3], Michele Burrello[1,3], Jesper Nygård[1], and Kasper Grove-Rasmussen[1]
[1]*Center for Quantum Devices, Niels Bohr Institute, University of Copenhagen, 2100 Copenhagen, Denmark*
[2]*Sino-Danish Center for Education and Research (SDC) SDC Building, Yanqihu Campus, University of Chinese Academy of Sciences, 380 Huaibeizhuang, Huairou District, 101408 Beijing, China and*
[3]*Niels Bohr International Academy, Niels Bohr Institute, University of Copenhagen, 2100 Copenhagen, Denmark*

## CONTENTS

I. Coulomb blockade structure 2

II. Negative differential conductance 2

III. Additional data on bias spectroscopy and temperature dependence 3

IV. Thermal model for superconducting island resonances 6

V. Zero-bias gate maps 7

VI. Additional data for Device B 8

References 12

## I. COULOMB BLOCKADE STRUCTURE

Figure. S1 shows high bias measurements for device A revealing Coulomb blockade structure for different setup configurations. The charging energy is found $E_\mathrm{c} \approx 0.5$ meV for setups I − V. Setup VI reveals characteristic dips of conductance owing to the Fano effect [S1, S2]. Different slopes of the Coulomb diamonds are owed to the different capacitances to the various leads.

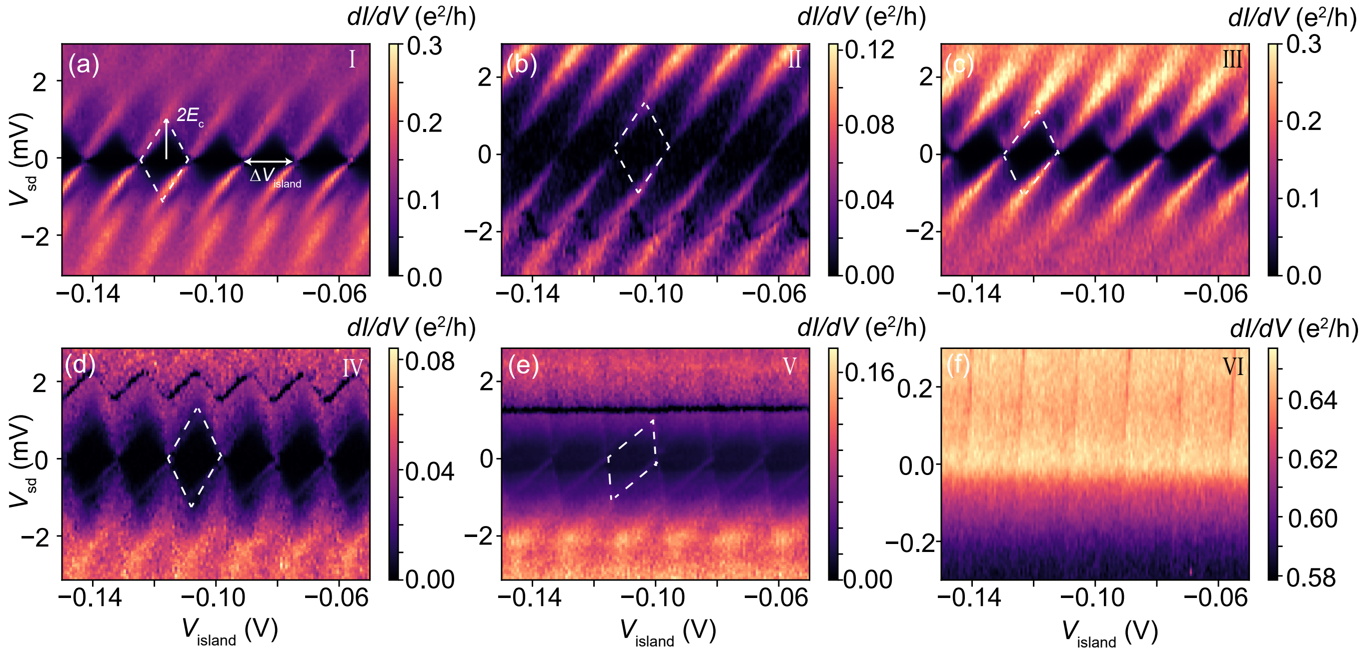


FIG. S1. Bias spectroscopy measurements for the six different setups. (a-e) Coulomb structure is observed in five setups yielding a charging energy $E_\mathrm{c} \approx 0.5$ meV. Dashed lines are a guide to the eye for the Coulomb diamonds. (f) No Coulomb structure observed, owing to the Fano effect. These measurements are taken in gate tuning $\alpha$.

## II. NEGATIVE DIFFERENTIAL CONDUCTANCE

In Fig. 3 of the main text, we observed a negative differential conductance (NDC) region in device A for odd charging of the SC island and finite bias, similarly to what has been reported in previous work on single nanowire blockaded devices [S3]. Typically, NDC features appear when there are excited states with a weaker coupling to the leads than the lowest energy state, which is responsible for transport at small biases. When a quasiparticle occupies the weakly coupled excited state, it slows down the transport process, thanks to the Coulomb blockade, and thus decreases the current flowing across the device. In Fig. S2, we focus in a single transport resonance between an odd and an even valley for device A and leads configuration I. Panels (a) and (b) compare the actual experimental measurement and the result of a rate equations calculation on a simplified three-state model, a trivial extension of the zero-bandwith model used in Ref. [S4]. The oblique lines in panel (b) indicate the conductance thresholds, where the voltage bias $V_\mathrm{sd}$ matches the energy differences between the many-body states involved in the sequential transport process. The three quasiparticle states considered in our model are: a low energy supgap state with energy $E_0$, a second excited subgap state with energy $E_1 > E_0$, and a state representing Bogoliubov quasiparticles above the SC gap with energy $\Delta$. Some of the physical parameters (subgap energy $E_0$, charging energy $E_c$, and SC gap $\Delta$) are taken from the experimental data, while $E_1$ is tuned to match the appearance of the NDC in the measurements. Many-body states are then labelled by their total charge $N$ and the occupation of the three quasiparticle states $|n_0, n_1, n_\Delta\rangle$. The lowest energy subgap state has a stronger coupling with the leads than the other two states. When a sequential tunneling event occurs, i.e. a particle is exchanged between one of the leads and the SC device, the total charge and the occupation number of a single quasiparticle state change by one.

In previous works [S3], it has been argued that the NDC appears when a particle occupies a QP state above the gap ($n_\Delta = 1$) and remains trapped there. However, this process is not consistent with our measurements because

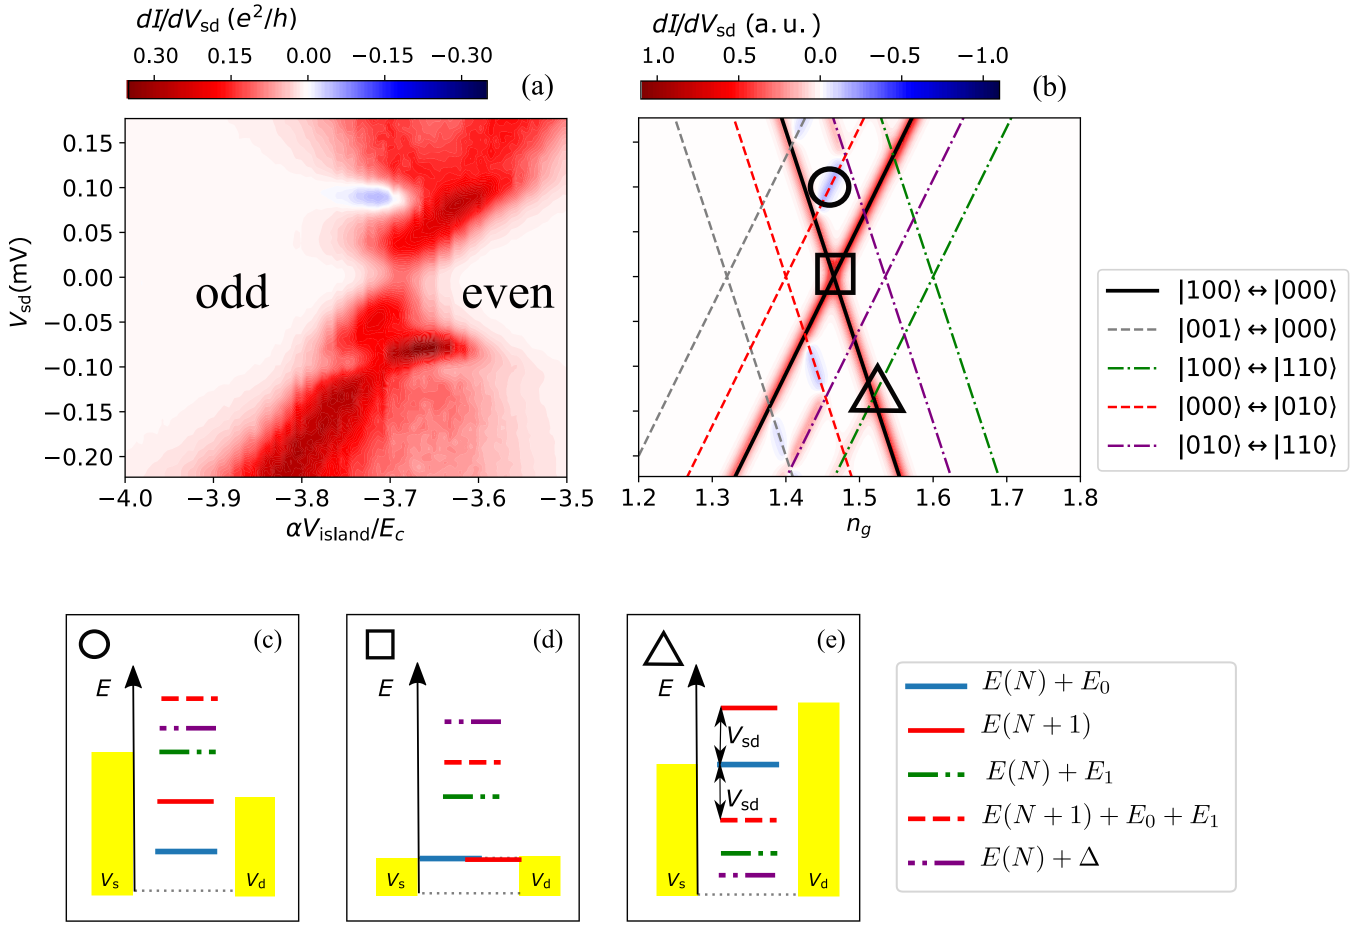


FIG. S2. (a): Differential conductance in the $V_{island}$-$V_{sd}$ plane for device A, setup III. The $x$-axis has been rescaled to the adimensional induced charge $n_g = \alpha V_{island}/E_c$, where $\alpha$ is the gate's lever arm, up to an offset. (b): rate equations result for the three state model. The energy of the second subgap state $E_1 \sim 0.1$meV has been tuned to match the position of the NDC with the experimental data, while the other physical parameters ($E_0$, $E_c$, $\Delta$) are extracted from the measurements. Oblique lines correspond to the resonances between possible transitions due to sequential tunneling events. (c)-(e): electrochemical schematics for three points in the $n_g - V_{sd}$ plane, highlighted in panel (b). the horizontal lines indicate the energy differences between the initial and final states involved in a sequential tunneling event. In these sketches we are assuming that drain voltage is aligned with the lowest energy state in the even sector (solid red line). In panel (e), the processes $|000\rangle \leftrightarrow |100\rangle$ and $|100\rangle \leftrightarrow |110\rangle$ are both activated because they are in resonance with the bias voltage. $N$ is the total charge of the odd valley.

it would appear at higher biases (dashed grey line, corresponding to the resonance $|000\rangle \leftrightarrow |001\rangle$), if we assume the $E_0 \simeq 35\mu$eV and $\Delta \simeq 180\mu$eV. A second subgap state with energy $E_1 \sim \Delta/2$ and weakly coupled to the leads, instead, leads to NDC in a range of voltage bias comparable to what measured in the experiments.

On a physical level, the presence of more subgap states can be expected in a device with complex geometry. In the simplest scenario, if each nanowire hosts a single subgap state, the hybridization due to the shared SC coating might induce some effective coupling between them. As a result, a possible degeneracy will be lifted and one supgap state ($E_0$) will be pushed further down in energy wile the other will be pushed up ($E_1$).

Panels (c)-(e) of fig. S2 sketch the electrochemical diagrams corresponding to three different points in the induced charge-voltage bias plane. Processes with and energy difference between the initial and final states below $V_{sd}$ are activated and contribute to transport, while those at higher energy do not.

## III. ADDITIONAL DATA ON BIAS SPECTROSCOPY AND TEMPERATURE DEPENDENCE

In this section we include the zero-bias traces for each setup measured in the superconducting and normal state ($B$= 0.4 T), bias spectroscopy maps (Fig. S3) magnetic field dependence measurements (Fig. S4) as well as the temperature dependence measurements (Fig. S5) for all six setups of Device A.

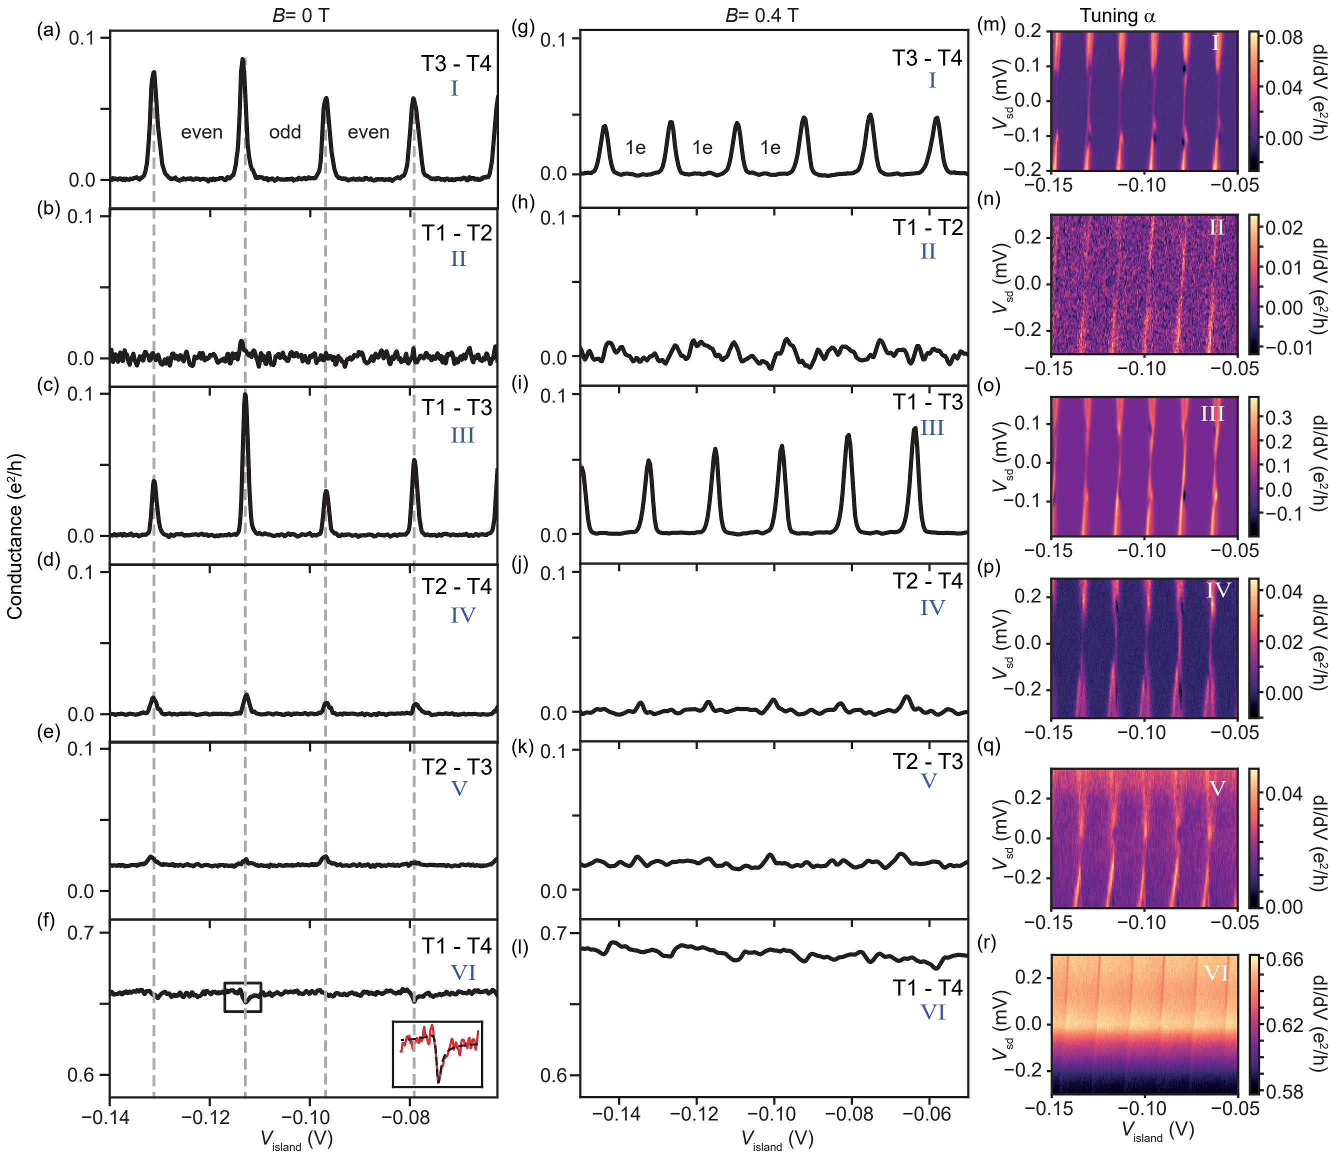

FIG. S3. (a-f) Zero-bias conductance traces as a function of gate for each two-terminal combination. (g-l) Zero-bias conductance traces measured in the normal (state $B$= 0.4 T) for each two-terminal combination. The peaks are misaligned across different setups due to gate switches that occur when sweeping the magnetic field. (m-r) Bias spectroscopy for each setup. Measurements taken in gate tuning $\alpha$.

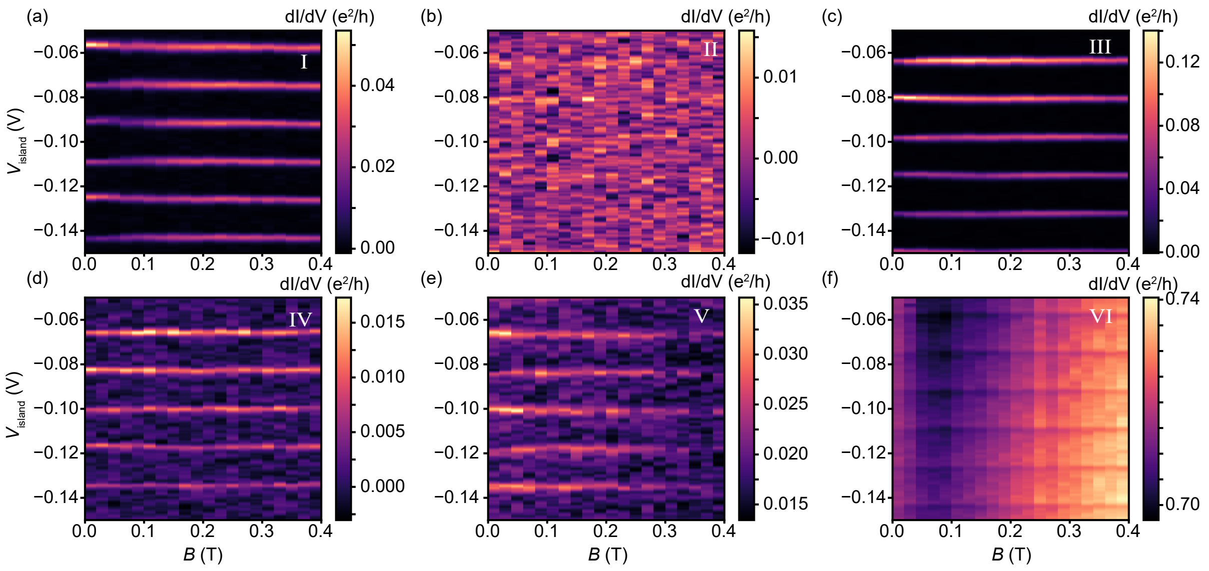


FIG. S4. (a-f) Zero bias magnetic field dependence of the superconducting island (SI) resonances. Measurements taken in gate tuning $\alpha$.

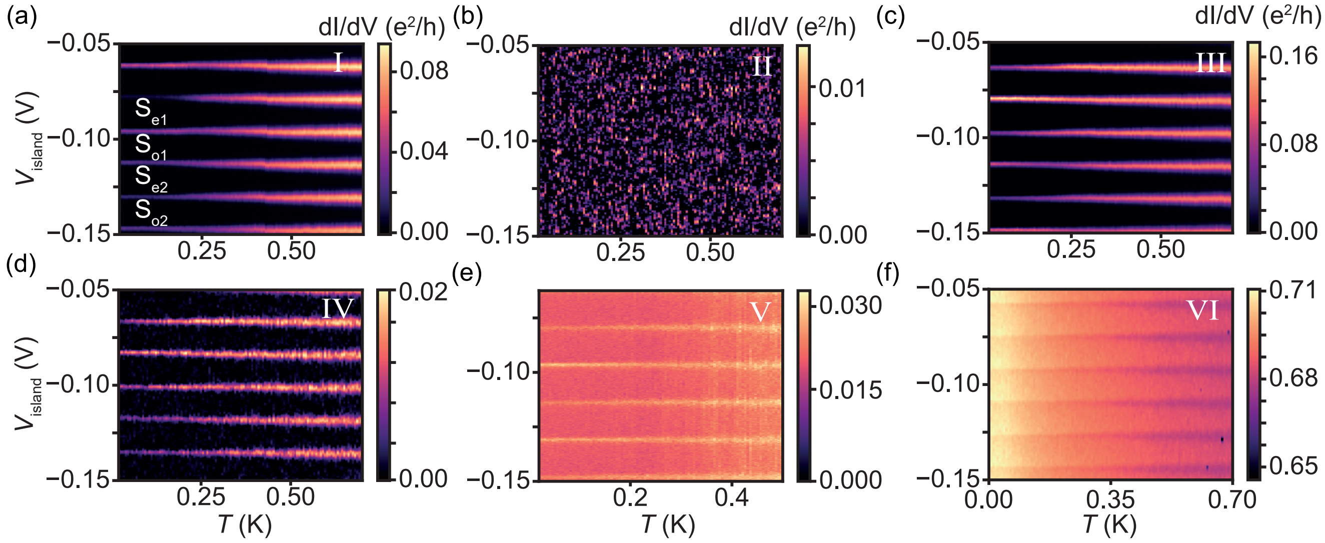


FIG. S5. (a-f) Zero bias temperature dependence of the superconducting island (SI) resonances. Measurements taken in gate tuning $\alpha$.

## IV. THERMAL MODEL FOR SUPERCONDUCTING ISLAND RESONANCES

The fitting of Fig. 4(c,d) (solid lines) is done by using eq. S1

$$F_\mathrm{o} - F_\mathrm{e} \approx -k_\mathrm{B}T \ \ln\, \tanh \left[ 2\rho_\mathrm{Al} V_\mathrm{Al} \Delta K_1 \left( \frac{\Delta}{k_\mathrm{B}T} \right) + \ln\, \coth \left( \frac{E_0}{2k_\mathrm{B}T} \right) \right] \tag{S1}$$

where $\rho_\mathrm{Al} = 23\ \mathrm{eV}^{-1}\ \mathrm{nm}^{-3}$ is the electron density of states of aluminum [S5–S7], $V_\mathrm{Al} = 91.8 \cdot 10^4\ \mathrm{nm}^3$ is the volume of the aluminum island, $K_1(x)$ is the Bessel function of the second kind, $\Delta$ is the superconducting gap of the island and $E_0$ is the lowest energy bound state originating by the proximity of InAs-Al. Using the above formula, we can extract a precise estimate of the energy of the bound state at different gate configurations, as shown in Fig. 4(b,c). The presence of a second subgap state with and energy $E_1 > E_0$ would add a term ln coth $\left(\frac{E_1}{2k_\mathrm{B}T}\right)$ inside the hyperbolic tangent. However, as long as $E_0$ and $E_1$ are clearly separated, its presence introduces negligible changes in the behavior of Eq. (S1), thus allowing for the estimating the lowest subgap energy $E_0$ from the measurements without using a more complex model.

In order to extract the number of quasiparticles in the SI, we need to define the saturation temperature $T_\mathrm{sat}$ which occurs when the the spacing difference starts to be modified. As shown in Fig. 4 of the main text, this temperature is $T_\mathrm{sat} = 140$ mK. We can now estimate the upper bound of $n_\mathrm{qp}$ for low temperatures which is given by eq. S2 where $N_\mathrm{eff} = \rho_\mathrm{Al} V_\mathrm{Al} \sqrt{2\pi k_\mathrm{B} T \Delta}$.

$$n_\mathrm{qp}(T) = V_\mathrm{Al}^{-1} N_\mathrm{eff}^2\ \mathrm{e}^{-2\Delta/(k_\mathrm{B}T)} \tag{S2}$$

Using eq. S2 we extract an upper bound of quasiparticle density $n_\mathrm{qp}(T_\mathrm{sat}) = 3.6\ \mu\mathrm{m}^{-3}$ for temperatures lower than 140 mK, which is reflected to an upper bound of number of quasiparticles $n_\mathrm{qp} V_\mathrm{Al} < 3 \cdot 10^{-3}$.

Figure. S6 shows spacing differences $\mathrm{S_e} - \mathrm{S_o}$ as a function of $T$ for finite magnetic field. Solid lines are fits using eq. S1. For higher $B$ the spacing diminishes, showing that the energy of the bound state has decreased due to the Zeeman effect. The raw data from where the spacings are extracted are shown in Fig. S7. This measurement proves that superconductivity is present for $B > 200$ mT.

Figure. S8 shows three different spacing differences extracted from Fig. S5a showing that across several charge states the change in the peaks is negligible, hinting that the SI parameters ($\Delta$, $E_0$) are not modified. The discrepancy at temperatures lower than 150 mK is owed to state broadening [S3] which is not included in the fits.

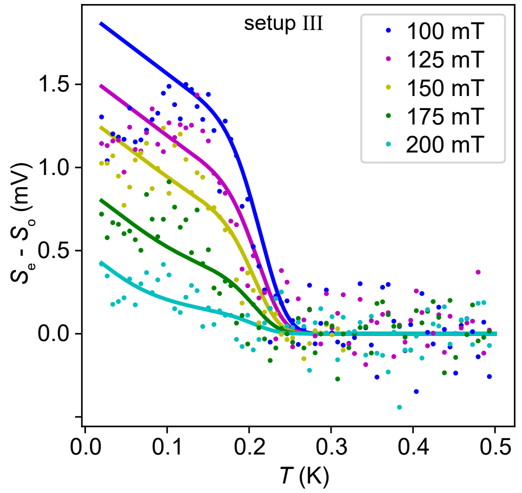


FIG. S6. Difference of even-odd sectors as a function of temperature for setup III at different magnetic field values.

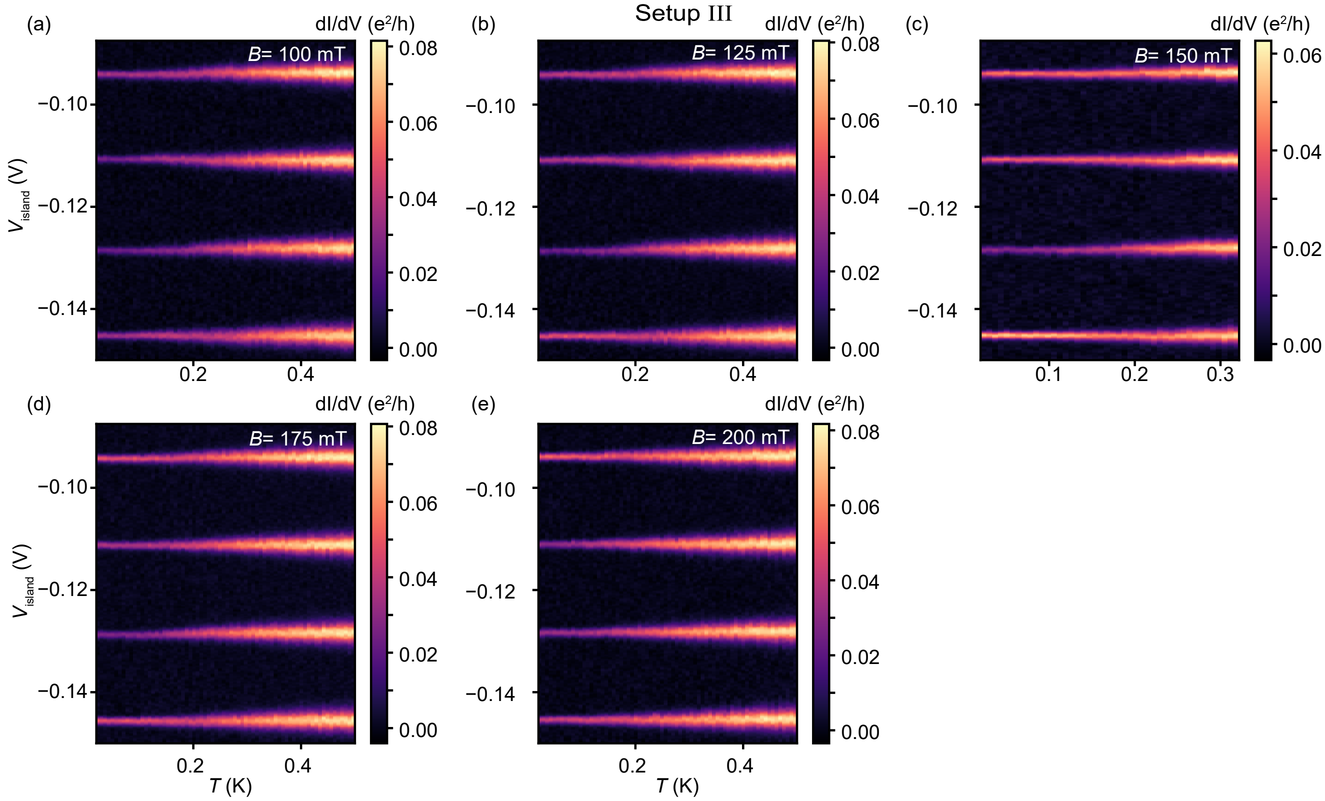


FIG. S7. Temperature dependence of the SI resonances at different magnetic field values. Data taken in setup III.

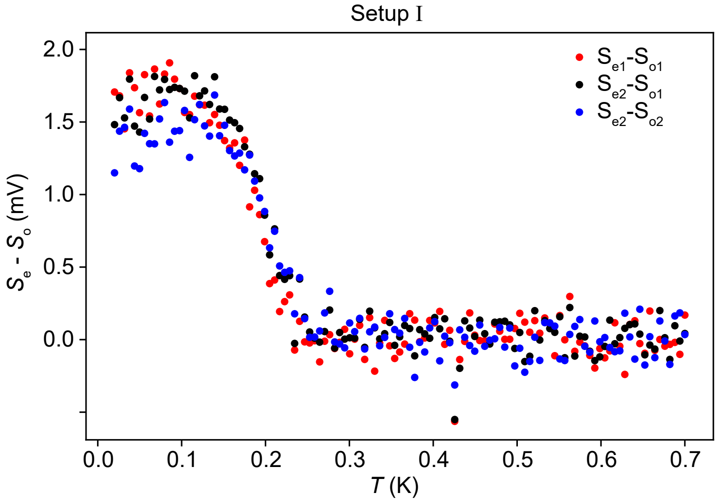


FIG. S8. Comparison of different even odd spacing differences. Legend corresponds to the $S_{\mathrm{e}}$, $S_{\mathrm{o}}$ of Fig. S5a. Data taken in setup I.

## V. ZERO-BIAS GATE MAPS

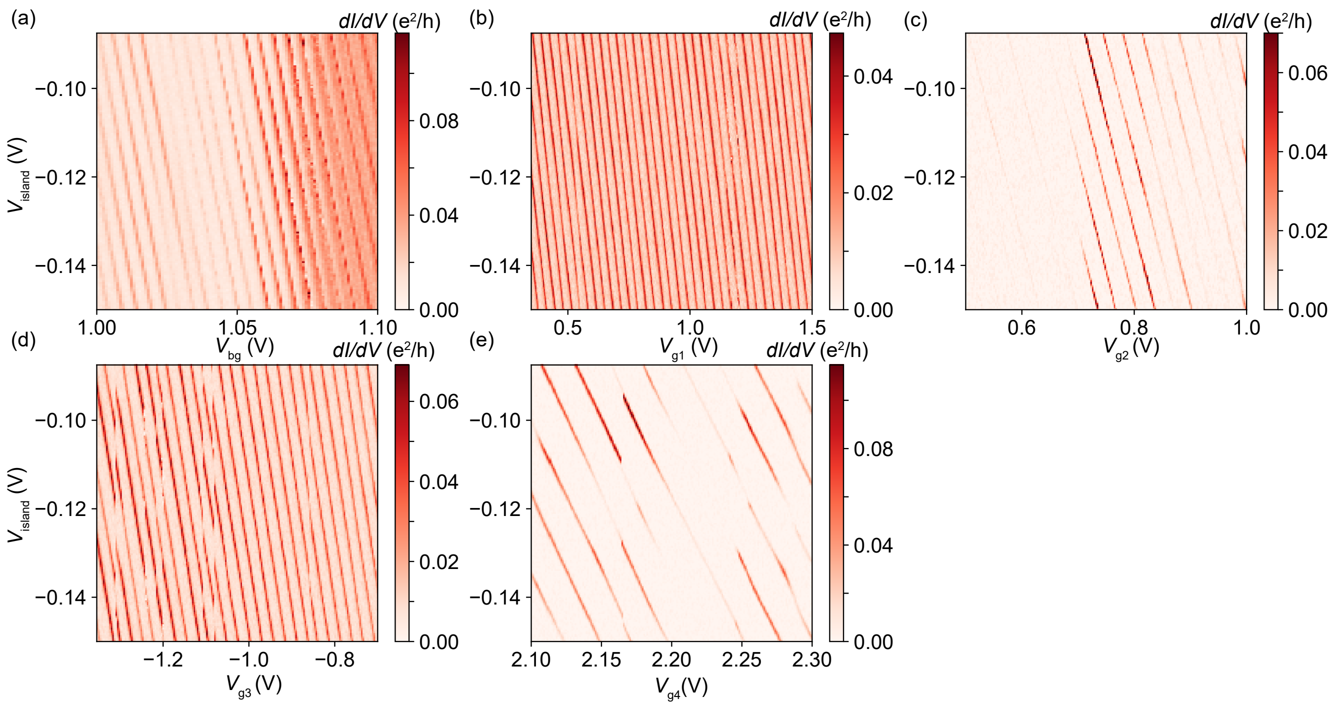


FIG. S9. Zero-bias maps of $V_{\mathrm{island}}$ as a function of every other gate of device A. No obvious signs of quantum dots are observed, apart from the regular resonances of the superconducting island across all gate combinations.

Figure S9 shows zero-bias conductance maps of the plunger gate tuning the SI versus each other gate of the device. All gate maps reveal regular resonances that belong to the superconducting island. In Figure. S9e shifts in the amplitude of the resonances are caused by an unknown effect. Hence, no obvious signs of quantum dot formation in the nanowires are observed.

## VI. ADDITIONAL DATA FOR DEVICE B

Figure S10 shows zero-bias traces for each setup combination measured in the superconducting (Fig. S10(a-f)) and in the normal state (Fig. S10(g-l)). It is evident that only in setups $\mathrm{I, IV, VI}$ SI resonances are observed in the superconducting state. The absence of the resonances in the other setup combinations is owed to the weak coupling between the corresponding probed leads and the SI. When superconductivity breaks down at a high enough magnetic field, these resonances are recovered as seen in Fig. S10(h,i). The interwire co-tunneling is found lower than in Device A, as the background conductance in setups $\mathrm{V, VI}$ is lower than the corresponding ones of Device A. The peaks are misaligned unlike Device A because these measurements were not taken directly one after another, as gate-switches cause small changes in the voltages where the resonances are measured. The magnetic field data were the above measurements were taken from are shown in Fig. S11. Figure S12 shows the method used to estimate $E_{\mathrm{c}}$ and $E_0$ for device B.

In a different gate configuration, Fig. S13 shows zero-bias traces as well as bias spectroscopy measurements for the six two-terminal combination setups for Device B. The signal is strongly suppressed inside the superconducting gap on most setups. However, Coulomb resonances are observed on all combinations confirming that the same SI is probed by all terminals.

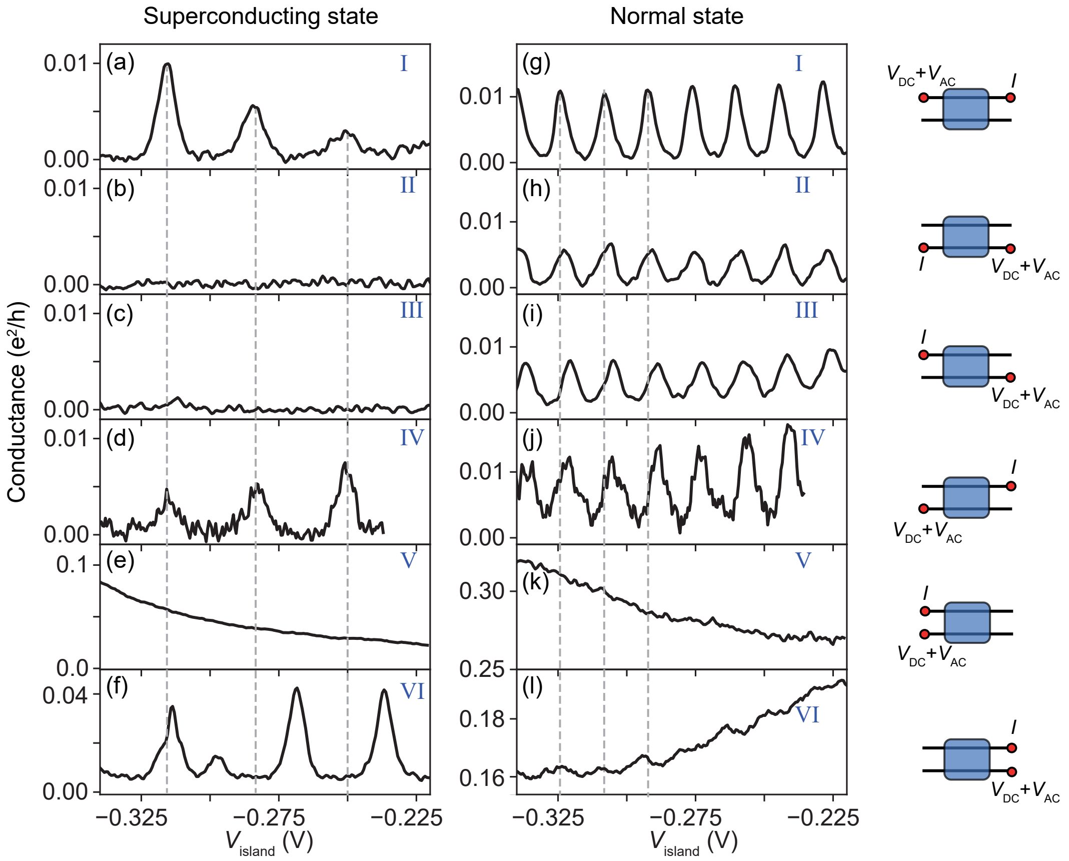


FIG. S10. Zero-bias conductance traces as a function of $V_{\mathrm{island}}$ for each two-terminal combination for Device B at the superconducting state ($B$= 0 T) and at the normal state ($B$= 0.5 T). Panel (l) is generated by averaging the signal for measurements from $B$= 0.3 T to $B$= 0.35 T.

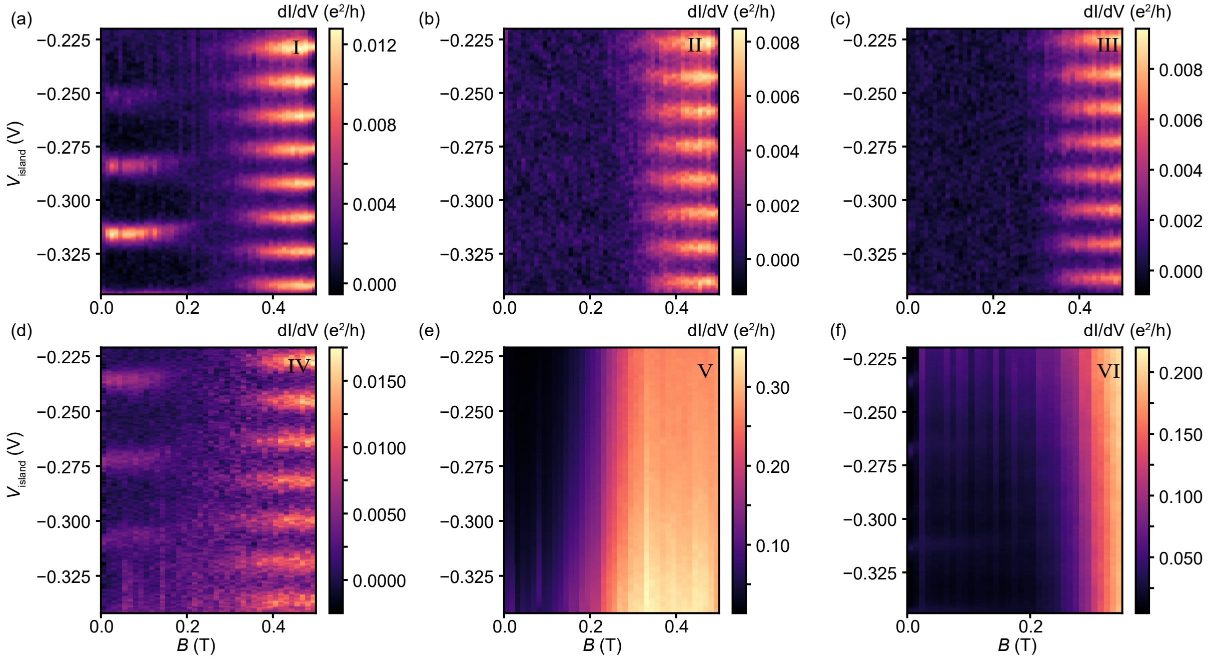


FIG. S11. (a-f) Zero bias magnetic field dependence of the superconducting island (SI) resonances in Device B. Data shown in Fig. S10 are generated by these panels.

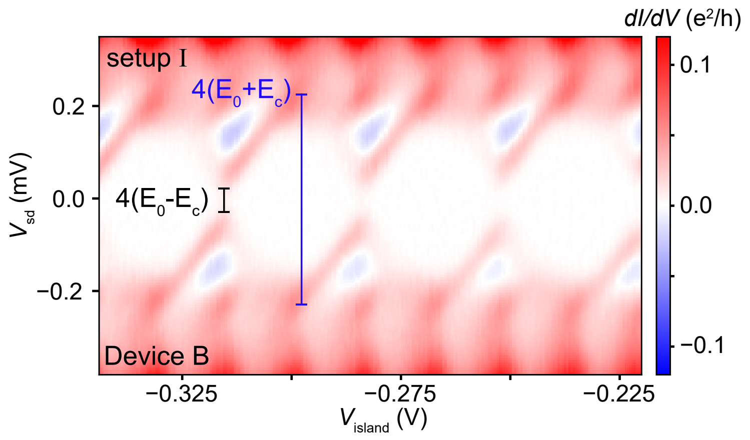


FIG. S12. Bias spectroscopy measurement of the SI in device B. As the SI is tuned at the $E_c < E_0$ regime, conductance in the proximity of zero-bias is suppressed (only valid for weakly coupled SI) and $4(E_0 - E_c)$ can be extracted from the black line. The distance between the tips of the diamonds (blue line) is $4(E_c + E_0)$. Therefore, the two values are estimated $E_c \approx 55$ $\mu$eV and $E_0 \approx 65$ $\mu$eV.

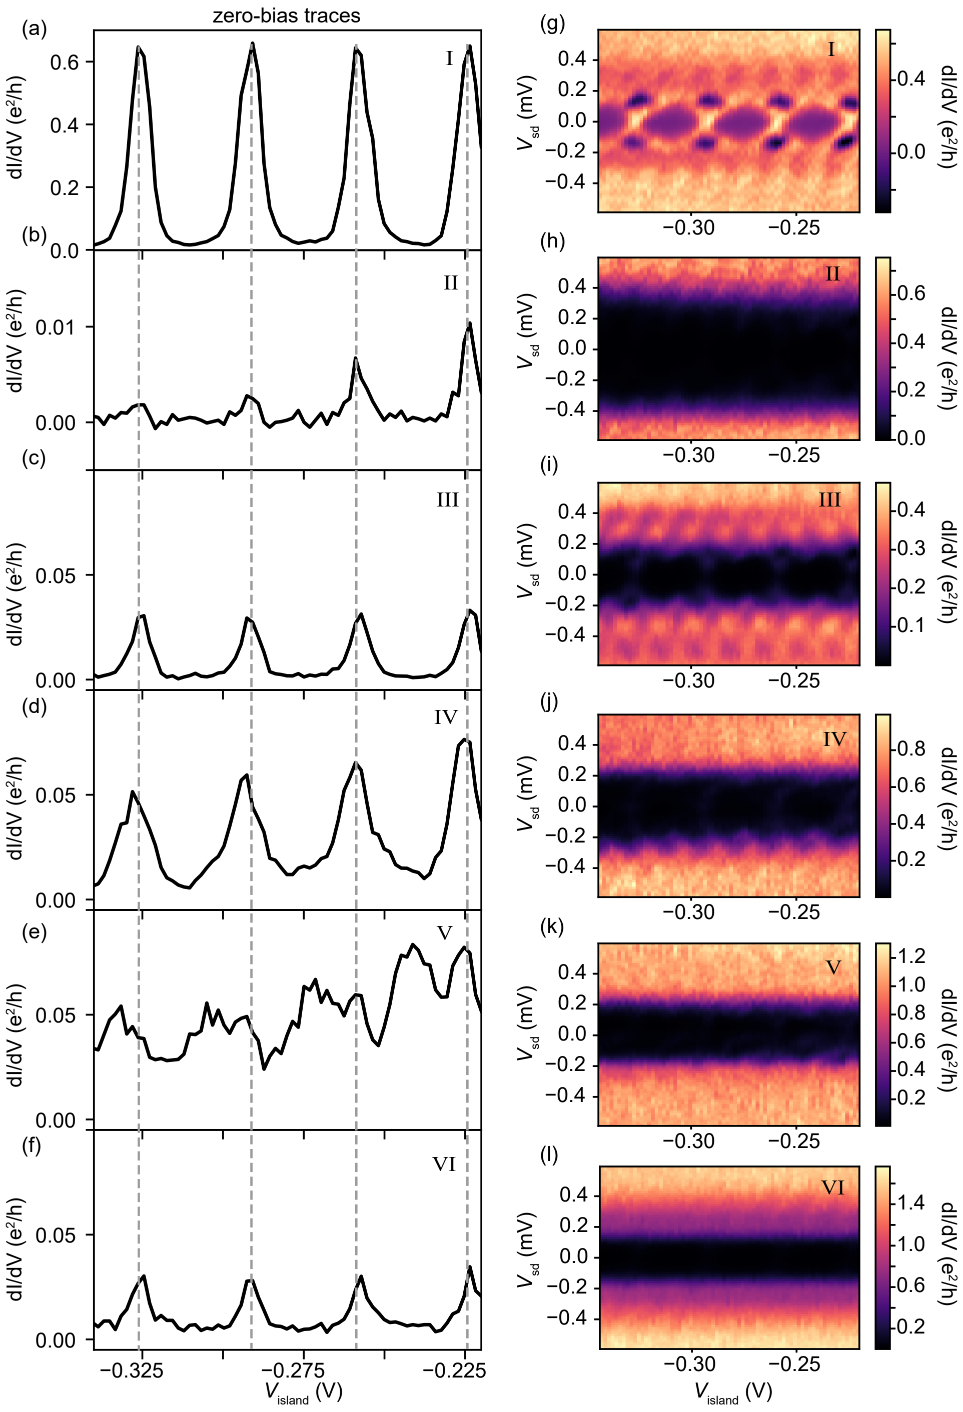


FIG. S13. Zero-bias traces for each two-terminal combination (a-f) with the corresponding bias spectroscopy measurements (g-l). The zero bias signal is strongly suppressed on all combinations but setup I. Above the superconducting gap higher conductance is recovered. Measurements are taken in a different gate configuration compared to the data shown in the main text.

[S1] U. Fano, "Effects of configuration interaction on intensities and phase shifts," Phys. Rev. **124**, 1866–1878 (1961).
[S2] B. Babić and C. Schönenberger, "Observation of fano resonances in single-wall carbon nanotubes," Phys. Rev. B **70**, 195408 (2004).
[S3] Andrew Patrick Higginbotham, Sven Marian Albrecht, Gediminas Kiršanskas, Willy Chang, Ferdinand Kuemmeth, Peter Krogstrup, Thomas Sand Jespersen, Jesper Nygård, Karsten Flensberg, and Charles M Marcus, "Parity lifetime of bound states in a proximitized semiconductor nanowire," Nature Physics **11**, 1017–1021 (2015).
[S4] S. Vaitiekėnas, R. Seoane Souto, Y. Liu, P. Krogstrup, K. Flensberg, M. Leijnse, and C. M. Marcus, "Evidence for spin-polarized bound states in semiconductor–superconductor–ferromagnetic-insulator islands," Phys. Rev. B **105**, L041304 (2022).
[S5] P. Lafarge, P. Joyez, D. Esteve, C. Urbina, and M. H. Devoret, "Measurement of the even-odd free-energy difference of an isolated superconductor," Phys. Rev. Lett. **70**, 994–997 (1993).
[S6] M. T. Tuominen, J. M. Hergenrother, T. S. Tighe, and M. Tinkham, "Experimental evidence for parity-based 2e periodicity in a superconducting single-electron tunneling transistor," Phys. Rev. Lett. **69**, 1997–2000 (1992).
[S7] V. F. Maisi, S. V. Lotkhov, A. Kemppinen, A. Heimes, J. T. Muhonen, and J. P. Pekola, "Excitation of single quasiparticles in a small superconducting al island connected to normal-metal leads by tunnel junctions," Phys. Rev. Lett. **111**, 147001 (2013).
